# Supplementary material for: Hybrid Discriminative Attribute-Object Embedding Network for Compositional Zero-Shot Learning
Source: arXiv:2412.00121 source file (2024-11-28)
Supplement: Supplementary file 1 [file X_suppl.tex]

\clearpage
\setcounter{page}{1}
\maketitlesupplementary
\section{Extended Experiment}
%\label{sec:rationale}
\subsection{Compared Methods}
We experiment with three CZSL benchmark datasets. To ensure fairness, we use the results of their published works for methods 1 to 6. For methods 6 to 16., we retrain the corresponding models on the corresponding datasets using the ViT-B backbone.
(1) CANet~\cite{wang2023learning} learns conditional attribute embeddings to compute attribute and object classification probabilities conditioned on images, thereby enhancing generalization.
(2) PSC-VD~\cite{li2024agree} reduces visual bias by exploring semantic consistency and proposes a multi-scale concept combination method to generate diverse virtual samples, enhancing the distinguishability and generalization ability of representation.
(3) CSCNet~\cite{zhang2024cscnet} designs a novel A-O disentanglement framework, namely, the Class-Specified Cascade Network.
(4) SAD-SP~\cite{liu2023simple} models dependencies through feasibility and context, and designs semantic attention and generative knowledge disentanglement.
(5) ProCC~\cite{huo2024procc} revisits traditional primitive prediction methods and introduces a progressive training approach, optimizing primitive classifiers on pre-trained features by moving from simpler to more challenging cases.
(6) OADis~\cite{Saini_2022_CVPR} generates complex concepts and optimizes recognition models by disentangling objects and attributes from visual features.
(7) IVR \cite{zhang2022learning} learns object-invariant features via cross-domain alignment for reliable attribute recognition.
(8) CompCos \cite{mancini2021open} maps image features to a semantic space using cosine similarity and improves training with feasibility scores.
(9) GraphEmbed \cite{naeem2021learning} learns image features and compositional representations end-to-end by leveraging dependencies in the graph structure to enhance generalization.
(10) SCEN~\cite{li2022siamese} creates virtual compositions via conjoined contrast spaces and state transition modules to diversify training.
(11) Co-CGE~\cite{mancini2022learning} enhances the model by considering embedding similarity of external semantic information and feasibility of graph structure.
(12) DLM~\cite{hu2024dynamic} proposes a realistic combinatorial zero-shot learning task and relabels MIT-States.
(13) ADE~\cite{hao2023learning} learns concept embeddings using cross-attention as a disentangler and regularizes feature similarity with EMD. 
(14) PBadv~\cite{li2024contextual} introduces a new oversampling strategy driven by object similarity to improve the training data for the target group.
(15) HPL~\cite{wang2023hierarchical} constructs three levels of hierarchical embedding spaces to represent states, objects, and their individual components separately.
(16) COT~\cite{kim2023hierarchical} uses object and attribute experts to generate representative embeddings, layer by layer using a visual network.

\subsection{Impact of the ratio $\alpha:\beta$}
\begin{figure}[!t]
\centering
    \includegraphics[width = \linewidth]{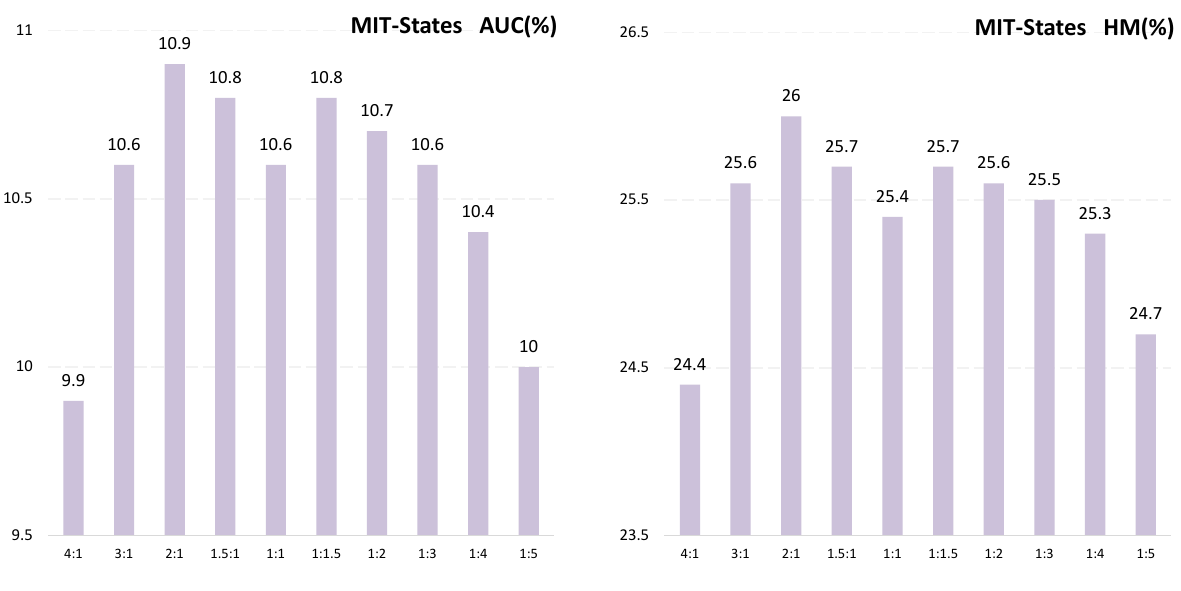}
    \caption{Effect of the ratio $\alpha:\beta$ on the MIT-States dataset.}
\label{ab}
\end{figure}
Figure \ref{ab} illustrates the effect of varying the ratio $\alpha:\beta$in the total loss function on the model's AUC and HM performance metrics for the MIT-States dataset. These metrics help assess the model's ability to generalize across diverse attribute-object combinations. The ratio $\alpha:\beta$ determines the relative contributions of the base loss $\mathcal{L}_{base}$, which focuses on overall classification accuracy, and the embedding loss $\mathcal{L}_{emd}$, which encourages better alignment and separation in the feature space. By adjusting this ratio, we can observe how different weightings affect the model's performance.
The results indicate that both AUC and HM reach their peak values at a ratio of $2:1$, with the highest AUC achieving 10.9\% and HM reaching 26\%. Ratios significantly higher or lower than $2:1$, such as $4:1$ or $1:5$, lead to noticeable declines in both metrics. This pattern suggests that an imbalance between $\mathcal{L}_{base}$ and $\mathcal{L}_{emd}$ can harm the model's learning capacity. Specifically, a higher weight on $\mathcal{L}_{base}$ may lead to an overemphasis on classification accuracy, potentially at the cost of fine-tuning the feature space alignment. On the other hand, giving too much weight to $\mathcal{L}_{emd}$ may result in excessive focus on embedding refinement, which could cause overfitting to specific features. Therefore, the $2:1$ ratio provides an optimal trade-off, allowing the model to balance accurate classification with robust feature alignment. This balanced approach ensures that the model can generalize effectively, achieving superior performance on compositional tasks in the MIT-States dataset, particularly in handling diverse and unseen attribute-object combinations.
%The results indicate that both AUC and HM reach their peak values at a ratio of $2:1$, with the highest AUC achieving 10.9\% and HM reaching 26\%. Ratios significantly higher or lower than $2:1$, such as $4:1$ or $1:5$, lead to noticeable declines in both metrics. This pattern suggests that an imbalance between $\mathcal{L}_{base}$ and $\mathcal{L}_{emd}$ diminishes the model's ability to learn and generalize effectively. The $2:1$ ratio thus provides an optimal trade-off between these two components, allowing the model to leverage both accurate baseline predictions and robust feature alignment. This balance enables better feature representation and generalization, resulting in improved performance on compositional tasks within the MIT-States dataset.

\subsection{Impact of the backbone network}
%We evaluated different backbone networks on the UT-Zappos dataset. In Table \ref{tablenetwork}, we studied the effects of fine-tuning and frozen feature extractors on model performance under both CW-CZSL and OW-CZSL settings, as well as the performance of two backbone networks: $ViT$ and $ResNet$. The results showed that $ViT$ is clearly more suitable for our model compared to ResNet. Under both CW and OW settings, all indicators for $Vit_{fine}$ are higher than for $Resnet_{fine}$, and all indicators for $Vit_{ff}$ are higher than for $Resnet_{ff}$. Moreover, after fine-tuning, both $ViT$ and $ResNet$ significantly outperform their frozen feature extractor counterparts, indicating that a fixed backbone network may not effectively extract visual information. The model using $Vit_{fine}$ as the backbone network performs best across all indicators. Under the closed-world setting, the AUC reached 38.4\%, HM was 54.0\%, and S and U were 63.4\% and 68.7\%, respectively. Under the open-world setting, the AUC reached 28.9\%, HM was 45.7\%, and S and U were 60.8\% and 54.9\%, respectively. %These results demonstrate that using $Vit_{fine}$ enhances the model's performance and generalization ability.
We evaluated different backbone networks on the UT-Zappos dataset to examine the impact of feature extraction techniques on model performance. In Table \ref{tablenetwork}, we explore the effects of fine-tuning and frozen feature extractors on performance in both the closed-world (CW-CZSL) and open-world (OW-CZSL) settings. We also compare two backbone networks: ViT and ResNet. The results indicate that ViT is more suitable for our model than ResNet. In both CW and OW settings, all performance indicators for $Vit_{fine}$ exceed those of $Resnet_{fine}$, and the performance of $Vit_{ff}$ is also higher than that of $Resnet_{ff}$. This suggests that fine-tuning ViT significantly improves results across the board compared to ResNet. Additionally, both ViT and ResNet show substantial improvements when fine-tuned, outperforming their frozen counterparts. This indicates that a fixed backbone network may not capture all necessary visual features effectively.
The model using $Vit_{fine}$ as the backbone achieves the best performance across all metrics. Under the closed-world setting, the AUC reached 38.4\%, HM was 54.0\%, and S and U were 63.4\% and 68.7\%, respectively. Under the open-world setting, AUC was 28.9\%, HM was 45.7\%, and S and U were 60.8\% and 54.9\%, respectively. These results confirm that using $Vit_{fine}$ significantly enhances the model’s performance and generalization ability, leading to improvements in all key metrics. This reinforces that ViT, when fine-tuned, is a more effective backbone than ResNet, especially for handling the hybrid and long-tail nature of the dataset. The superior performance of $Vit_{fine}$ highlights the importance of using a flexible backbone that can adapt to varying data distributions and task-specific challenges.

\begin{table}[!t]
    \centering
    \resizebox{\linewidth}{!}{
        \begin{tabular}{c|c|cccccc}
        \hline
        \multirow{2}{*}{} & \multirow{2}{*}{Backbone} & \multicolumn{6}{c}{UT-Zappos 50K}\\
        \cline{3-8}
        & & AUC & HM & S & U & A & O\\
        \hline
        \multirow{3}{*}{Close}
        & $Resnet_{ff}$&24.7&42.2&55.6&51.9&37.0&63.2\\
        & $Resnet_{fine}$ & 35.5 & 51.5 & 59.5 & 66.9 & 47.7 & 71.8\\
        & $Vit_{ff}$ & 28.3 & 44.7 & 54.4 & 61.2 & 44.3 & 69.3\\
        &$Vit_{fine}$ & \textbf{38.4}&\textbf{54.0}&\textbf{63.4}&\textbf{68.7}& \textbf{49.2} & \textbf{76.2}\\
        \hline
        \multirow{3}{*}{Open}
        & $Resnet_{ff}$&16.1&33.1&52.9&37.6&28.8&64.7\\
        & $Resnet_{fine}$&25.3&42.6&59.5&50.9&37.2&73.6\\
        & $Vit_{ff}$ &19.7&37.4&50.1&47.7&35.5&69.6\\
        & $Vit_{fine}$ &\textbf{28.9}&\textbf{45.7}&\textbf{60.8}&\textbf{54.9}&\textbf{40.4}&\textbf{75.8}\\
        \hline
        \end{tabular}
    }
    \caption{ The performance metrics of the UT-Zappos dataset under different backbone networks, and we bold the optimal values on the table.}
\label{tablenetwork}
\end{table}

\subsection{Impact of word embedding models}
Table \ref{tableglove} presents the performance of various word embedding models on the UT-Zappos 50K dataset, comparing FastText ($ft$), GloVe ($gl$), and Word2Vec ($w2v$), both individually and in combination. When used individually, GloVe outperforms the other models in key metrics, including AUC and HM, demonstrating its strong ability to capture and represent attribute-object combinations. On the other hand, FastText achieves higher scores in S and U, which correspond to known and unknown attribute-object combinations, respectively. However, its relatively lower HM score suggests that the model may struggle with balancing these combinations effectively. Word2Vec yields moderate performance across the different metrics, delivering consistent and stable results, but not as outstanding as GloVe in terms of AUC and HM.
When combining the word embedding models, such as $ft + w2v$ or $gl + ft$, the dimensionality increases to 600 or even 900. However, the overall performance does not see significant improvements, and in some cases, there is a slight decline compared to using individual models. This can be attributed to the introduction of redundant information, which adds complexity to the feature space and may hinder the model's ability to generalize effectively to complex combinations. Specifically, when the three embeddings ($ft + w2v + gl$) are combined to form a 900-dimensional feature space, there is only a minor improvement in the S metric. Core indicators like HM and AUC show no significant gains, which suggests that simply increasing the number of embedding models or dimensions does not necessarily enhance model performance. Instead, the increased feature redundancy may even impair the model’s generalization ability.
Given these observations, the smaller and more efficient GloVe model strikes the best balance between performance and computational efficiency. It consistently provides strong performance while avoiding the pitfalls of higher-dimensional feature spaces. Therefore, we choose the GloVe model to generate word vectors in our approach, as it offers both strong representation of attribute-object relationships and computational practicality.
\begin{table}[!t]
    \centering
    \resizebox{\linewidth}{!}{
        \begin{tabular}{c|c|cccccc}
        \hline
         \multirow{2}{*}{Word Embedding} & \multirow{2}{*}{Dim}&\multicolumn{6}{c}{UT-Zappos 50K}\\
        \cline{3-8}
        & & AUC & HM & S & U & A & O\\
        \hline
        $ft$ & \multirow{3}{*}{300} &35.3 &49.5 &63.6 & \textbf{69.9}  & \textbf{49.6}  & \textbf{78.1}  \\
	$gl$ &  &\textbf{38.4} &\textbf{54.0} &63.4 &68.7 &49.2 &76.2\\
	$w2v$ & &35.9 &52.8 &63.9  & 68.5  & 48.9  & 77.5  \\
 \hline
	$ft+w2v$ &\multirow{7}{*}{600}&36.2 &50.6 &63.5 &69.0 & 48.7  & 76.8  \\
	$ft+gl$ & &35.9 &50.1 &61.9 &68.9  & 48.6  & 75.6  \\
	$gl+w2v$ &  &35.9 &52.5 &61.6 &68.7 & 48.7  & 75.5  \\
	$gl+ft$ & &37.2 &51.0 & 60.8 & 69.0 & 48.5  & 75.8  \\
	$gl+gl$ & &36.0 &50.7 & 61.6 & 68.8 & 48.2  & 76.0  \\
	$ft+ft$ & &35.8 &50.5 & 62.4 & 68.8 & 48.4  & 76.3  \\
	$w2v+w2v$ &  & 35.9 &51.4 &61.7 &66.9 & 47.3 & 76.6  \\
 \hline
	$ft+w2v+gl$ & 900&36.2 &50.6 &\textbf{64.7} &66.9 & 47.7  & 76.5 \\
        \hline
        \end{tabular}
    }
    \caption{ Performance indicators of the UT-Zappos dataset under different word embedding models. We mark the optimal values in bold in the table.}
\label{tableglove}
\end{table}
